# Supplementary material for: The Crewther relation, schemes, gauges and fixed points
Source: arXiv:2306.11416 ancillary file (2023-08-03)
Supplement: Supplementary file 1 [file qcdcrewspm.pdf]

## Supplementary Material.

| Linear Covariant Gauge and $\overline{\text{MS}}$ scheme |      |                |                 |            |                 |
|----------------------------------------------------------|------|----------------|-----------------|------------|-----------------|
| $N_f$                                                    | Loop | $\bar{\alpha}$ |                 | [42]       |                 |
|                                                          |      | $a_\infty$     | $\alpha_\infty$ | $a_\infty$ | $\alpha_\infty$ |
| 8                                                        | 3    | 0.116505       | 1.519357        | 0.116505   | -0.384782       |
|                                                          | 4    | 0.123312       | 1.644675        | 0.123312   | 0.868700        |
|                                                          | 4    | 1.142863       | 95.371427       | 1.142863   | 2.015974        |
| 9                                                        | 2    | 0.416667       | -1.958333       | 0.416667   | -2.146730       |
|                                                          | 3    | 0.081803       | -0.166164       | 0.081803   | -0.858773       |
|                                                          | 4    | 0.085291       | -0.309521       | 0.085291   | 0.078057        |
|                                                          | 4    | 0.962002       | -183.792290     | 0.962002   | -2.710372       |
| 10                                                       | 2    | 0.175676       | -2.268018       | 0.175676   | -2.303972       |
|                                                          | 3    | 0.060824       | -1.034992       | 0.060824   | -1.298293       |
|                                                          | 4    | 0.064860       | -1.096595       | 0.064860   | -0.758788       |
|                                                          | 4    | 0.446940       | -11.160925      | 0.446940   | -2.802990       |
| 11                                                       | 2    | 0.098214       | -2.427083       | 0.098214   | -2.432707       |
|                                                          | 3    | 0.046039       | -1.597571       | 0.046039   | -1.692825       |
|                                                          | 4    | 0.049832       | -1.606862       | 0.049832   | -1.444524       |
|                                                          | 4    | 0.262159       | 2.394487        | 0.262159   | 2.797166        |
| 12                                                       | 2    | 0.060000       | -2.550000       | 0.060000   | -2.548046       |
|                                                          | 3    | 0.034607       | -2.010094       | 0.034607   | -2.039860       |
|                                                          | 4    | 0.037434       | -2.004044       | 0.037434   | -1.945284       |
|                                                          | 4    | 0.182641       | 2.526630        | 0.182641   | 2.874023        |

Table SM.1: Fixed points solutions for  $a_\infty$  and  $\alpha_\infty$  to the curve  $\gamma_a(a, \bar{\alpha}) = -\gamma_\alpha(a, \bar{\alpha})$ , in the columns headed with  $\bar{\alpha}$  and the corresponding solutions for the fixed points in the  $(a, \alpha)$ -plane given in [42], to four loops in the  $\overline{\text{MS}}$  scheme for the linear covariant gauge for  $8 \leq N_f \leq 12$ . There were no five loop solutions.

| Linear Covariant Gauge and $\overline{\text{MS}}$ scheme |      |                |                 |            |                 |
|----------------------------------------------------------|------|----------------|-----------------|------------|-----------------|
|                                                          |      | $\bar{\alpha}$ |                 | [42]       |                 |
| $N_f$                                                    | Loop | $a_\infty$     | $\alpha_\infty$ | $a_\infty$ | $\alpha_\infty$ |
| 13                                                       | 2    | 0.037234       | -2.658688       | 0.037234   | -2.655694       |
|                                                          | 3    | 0.025191       | -2.332918       | 0.025191   | -2.339613       |
|                                                          | 4    | 0.026853       | -2.328809       | 0.026853   | -2.312632       |
|                                                          | 4    | 0.141687       | 1.725784        | 0.141687   | 2.881045        |
|                                                          | 5    | 0.032315       | -2.412804       | 0.032315   | -2.386609       |
|                                                          | 5    | 0.041343       | -2.517612       | 0.041343   | -2.470802       |
| 14                                                       | 2    | 0.022124       | -2.760324       | 0.022124   | -2.758253       |
|                                                          | 3    | 0.017070       | -2.591444       | 0.017070   | -2.591922       |
|                                                          | 4    | 0.017793       | -2.591328       | 0.017793   | -2.588296       |
|                                                          | 4    | 0.117756       | 1.077329        | 0.117756   | 2.842775        |
|                                                          | 5    | 0.018526       | -2.605752       | 0.018526   | -2.603426       |
|                                                          | 5    | 0.046357       | -2.868367       | 0.046357   | -2.932818       |
| 15                                                       | 2    | 0.011364       | -2.857955       | 0.011364   | -2.857085       |
|                                                          | 3    | 0.009818       | -2.795342       | 0.009818   | -2.795125       |
|                                                          | 4    | 0.010001       | -2.796093       | 0.010001   | -2.795819       |
|                                                          | 4    | 0.102368       | 0.613815        | 0.102368   | 2.778768        |
|                                                          | 5    | 0.010078       | -2.798028       | 0.010078   | -2.797897       |
|                                                          | 5    | 0.047107       | -3.112058       | 0.047107   | -3.326390       |
| 16                                                       | 2    | 0.003311       | -2.953091       | 0.003311   | -2.952985       |
|                                                          | 3    | 0.003162       | -2.945856       | 0.003162   | -2.945839       |
|                                                          | 4    | 0.003170       | -2.945937       | 0.003170   | -2.945935       |
|                                                          | 4    | 0.091700       | 0.277696        | 0.091700   | 2.700828        |
|                                                          | 5    | 0.003171       | -2.945966       | 0.003171   | -2.945965       |
|                                                          | 5    | 0.046999       | -3.321284       | 0.046999   | -3.682521       |

Table SM.2: Fixed points solutions for  $a_\infty$  and  $\alpha_\infty$  to the curve  $\gamma_a(a, \bar{\alpha}) = -\gamma_\alpha(a, \bar{\alpha})$ , in the columns headed with  $\bar{\alpha}$  and the corresponding solutions for the fixed points in the  $(a, \alpha)$ -plane given in [42], to five loops in the  $\overline{\text{MS}}$  scheme for the linear covariant gauge for  $13 \leq N_f \leq 16$ .

| Curci-Ferrari Gauge and $\overline{\text{MS}}$ scheme |      |                |                 |            |                 |
|-------------------------------------------------------|------|----------------|-----------------|------------|-----------------|
|                                                       |      | $\bar{\alpha}$ |                 | [42]       |                 |
| $N_f$                                                 | Loop | $a_\infty$     | $\alpha_\infty$ | $a_\infty$ | $\alpha_\infty$ |
| 8                                                     | 3    | 0.116505       | 5.425313        | 0.116505   | -0.525277       |
| 9                                                     | 2    | 0.416667       | 7.333333        | 0.416667   | -2.387888       |
|                                                       | 3    | 0.081803       | 1.386711        | 0.081803   | -1.239118       |
| 10                                                    | 2    | 0.175676       | 0.207207        | 0.175676   | -2.981627       |
|                                                       | 3    | 0.060824       | -0.762250       | 0.060824   | -1.988405       |
| 11                                                    | 2    | 0.098214       | -2.202381       | 0.098214   | -3.548192       |
|                                                       | 3    | 0.046039       | -2.180305       | 0.046039   | -2.744498       |
| 12                                                    | 2    | 0.060000       | -3.480000       | 0.060000   | -4.078489       |
|                                                       | 3    | 0.034607       | -3.235417       | 0.034607   | -3.479125       |
| 13                                                    | 2    | 0.037234       | -4.312057       | 0.037234   | -4.569040       |
|                                                       | 3    | 0.025191       | -4.075904       | 0.025191   | -4.169158       |
| 14                                                    | 2    | 0.022124       | -4.923304       | 0.022124   | -5.020489       |
|                                                       | 3    | 0.017070       | -4.768441       | 0.017070   | -4.796907       |
| 15                                                    | 2    | 0.011364       | -5.409091       | 0.011364   | -5.435844       |
|                                                       | 3    | 0.009818       | -5.342638       | 0.009818   | -5.347954       |
| 16                                                    | 2    | 0.003311       | -5.816777       | 0.003311   | -5.819105       |
|                                                       | 3    | 0.003162       | -5.808281       | 0.003162   | -5.808458       |

Table SM.3: Fixed points solutions for  $a_\infty$  and  $\alpha_\infty$  to the curve  $\gamma_a(a, \bar{\alpha}) = -\gamma_\alpha(a, \bar{\alpha})$ , in the columns headed with  $\bar{\alpha}$  and the corresponding solutions for the fixed points in the  $(a, \alpha)$ -plane given in [42], to three loops in the  $\overline{\text{MS}}$  scheme for the Curci-Ferrari gauge for  $8 \leq N_f \leq 16$ .

| MAG and $\overline{\text{MS}}$ Scheme |      |                |                 |            |                 |
|---------------------------------------|------|----------------|-----------------|------------|-----------------|
|                                       |      | $\bar{\alpha}$ |                 | [42]       |                 |
| $N_f$                                 | Loop | $a_\infty$     | $\alpha_\infty$ | $a_\infty$ | $\alpha_\infty$ |
| 8                                     | 3    | 0.116505       | -14.454928      | 0.116505   | -14.732061      |
| 9                                     | 2    | 0.416667       | -5.748610       | 0.416667   | -1.775685       |
|                                       | 3    | 0.081803       | -9.342567       | 0.081803   | -6.679483       |
| 10                                    | 2    | 0.175676       | -5.644755       | 0.175676   | -2.041475       |
|                                       | 3    | 0.060824       | -7.302268       | 0.060824   | -9.374058       |
| 11                                    | 2    | 0.098214       | -5.611372       | 0.098214   | -2.385628       |
|                                       | 3    | 0.046039       | -6.350328       | 0.046039   | -1.943195       |
| 12                                    | 2    | 0.060000       | -5.594904       | 0.060000   | -2.822900       |
|                                       | 3    | 0.034607       | -5.885931       | 0.034607   | -2.691103       |
| 13                                    | 2    | 0.037234       | -5.585093       | 0.037234   | -3.356225       |
|                                       | 3    | 0.025191       | -5.668820       | 0.025191   | -3.414438       |
| 14                                    | 2    | 0.022124       | -5.578581       | 0.022124   | -3.968278       |
|                                       | 3    | 0.017070       | -5.583155       | 0.017070   | -4.074876       |
| 15                                    | 2    | 0.011364       | -5.573944       | 0.011364   | -4.620179       |
|                                       | 3    | 0.009818       | -5.563763       | 0.009818   | -4.684705       |
| 16                                    | 2    | 0.003311       | -5.570474       | 0.003311   | -5.263519       |
|                                       | 3    | 0.003162       | -5.568155       | 0.003162   | -5.273175       |

Table SM.4: Fixed points solutions for  $a_\infty$  and  $\alpha_\infty$  to the curve  $\alpha\gamma_a(a, \bar{\alpha}) = -\alpha\gamma_\alpha(a, \bar{\alpha})$ , in the columns headed with  $\bar{\alpha}$  and the corresponding solutions for the fixed points in the  $(a, \alpha)$ -plane given in [42], to three loops in the  $\overline{\text{MS}}$  scheme for the MAG for  $8 \leq N_f \leq 16$ .

| Linear Covariant Gauge and RI' Scheme |      |                |                 |            |                 |
|---------------------------------------|------|----------------|-----------------|------------|-----------------|
|                                       |      | $\bar{\alpha}$ |                 | [42]       |                 |
| $N_f$                                 | Loop | $a_\infty$     | $\alpha_\infty$ | $a_\infty$ | $\alpha_\infty$ |
| 8                                     | 3    | 0.116505       | -21.994002      | 0.116505   | 2.038116        |
|                                       | 4    | 0.123312       | -90.871325      | 0.123312   | 1.454078        |
|                                       | 4    | 1.142863       | -54744.701936   | 1.142863   | 1.310571        |
| 9                                     | 2    | 0.416667       | -13.578704      | 0.416667   | 3.457480        |
|                                       | 3    | 0.081803       | -13.552345      | 0.081803   | 2.306390        |
|                                       | 4    | 0.085291       | -32.540125      | 0.085291   | 1.577736        |
|                                       | 4    | 0.962002       | -27258.566577   | 0.962002   | -4.785856       |
| 10                                    | 2    | 0.175676       | -7.640224       | 0.175676   | 3.922004        |
|                                       | 3    | 0.060824       | -9.167126       | 0.060824   | 2.571364        |
|                                       | 4    | 0.064860       | -14.944765      | 0.064860   | 1.682620        |
|                                       | 4    | 0.446940       | -1912.058570    | 0.446940   | -5.607503       |
| 11                                    | 2    | 0.098214       | -5.597828       | 0.098214   | 4.460256        |
|                                       | 3    | 0.046039       | -6.555838       | 0.046039   | 2.896474        |
|                                       | 4    | 0.049832       | -7.617584       | 0.049832   | -4.929912       |
|                                       | 4    | 0.262159       | -167.317558     | 0.262159   | -5.991881       |
| 12                                    | 2    | 0.060000       | -4.530000       | 0.060000   | 5.152191        |
|                                       | 3    | 0.034607       | -4.940648       | 0.034607   | 3.348119        |
|                                       | 4    | 0.037434       | -4.594412       | 0.037434   | -3.483133       |
|                                       | 4    | 0.182641       | 32.357517       | 0.182641   | -6.272709       |

Table SM.5: Fixed points solutions for  $a_\infty$  and  $\alpha_\infty$  to the curve  $\gamma_a(a, \bar{\alpha}) = -\gamma_\alpha(a, \bar{\alpha})$ , in the columns headed with  $\bar{\alpha}$  and the corresponding solutions for the fixed points in the  $(a, \alpha)$ -plane given in [42], to five loops in the RI' scheme for the linear covariant gauge for  $8 \leq N_f \leq 12$ .

| Linear Covariant Gauge and RI' Scheme |      |                |                 |            |                 |
|---------------------------------------|------|----------------|-----------------|------------|-----------------|
|                                       |      | $\bar{\alpha}$ |                 | [42]       |                 |
| $N_f$                                 | Loop | $a_\infty$     | $\alpha_\infty$ | $a_\infty$ | $\alpha_\infty$ |
| 13                                    | 2    | 0.037234       | -3.877298       | 0.037234   | 6.124282        |
|                                       | 3    | 0.025191       | -3.961680       | 0.025191   | -4.223426       |
|                                       | 4    | 0.026853       | -3.506328       | 0.026853   | -3.183587       |
|                                       | 4    | 0.141687       | 62.029508       | 0.141687   | -6.499993       |
|                                       | 5    | 0.032315       | -2.076171       | 0.032315   | -1.726095       |
|                                       | 5    | 0.041343       | 0.616996        | 0.041343   | -6.275659       |
| 14                                    | 2    | 0.022124       | -3.456544       | 0.022124   | -3.669491       |
|                                       | 3    | 0.017070       | -3.410161       | 0.017070   | -3.421636       |
|                                       | 4    | 0.017793       | -3.179254       | 0.017793   | -3.110067       |
|                                       | 4    | 0.117756       | 64.519521       | 0.117756   | -6.692429       |
|                                       | 5    | 0.018526       | -3.019295       | 0.018526   | -2.998799       |
|                                       | 5    | 0.046357       | 5.856563        | 0.046357   | -6.408426       |
| 15                                    | 2    | 0.011364       | -3.190025       | 0.011364   | -3.217291       |
|                                       | 3    | 0.009818       | -3.139610       | 0.009818   | -3.136331       |
|                                       | 4    | 0.010001       | -3.082196       | 0.010001   | -3.074901       |
|                                       | 4    | 0.102368       | 61.825485       | 0.102368   | -6.858264       |
|                                       | 5    | 0.010078       | -3.071347       | 0.010078   | -3.071076       |
|                                       | 5    | 0.047107       | 7.944044        | 0.047107   | -6.462481       |
| 16                                    | 2    | 0.003311       | -3.039142       | 0.003311   | -3.040393       |
|                                       | 3    | 0.003162       | -3.029633       | 0.003162   | -3.029389       |
|                                       | 4    | 0.003170       | -3.027390       | 0.003170   | -3.027317       |
|                                       | 4    | 0.091700       | 58.084238       | 0.091700   | -7.001486       |
|                                       | 5    | 0.003171       | -3.027349       | 0.003171   | -3.027350       |
|                                       | 5    | 0.046999       | 7.849534        | 0.046999   | -6.454812       |

Table SM.6: Fixed points solutions for  $a_\infty$  and  $\alpha_\infty$  to the curve  $\gamma_a(a, \bar{\alpha}) = -\gamma_\alpha(a, \bar{\alpha})$ , in the columns headed with  $\bar{\alpha}$  and the corresponding solutions for the fixed points in the  $(a, \alpha)$ -plane given in [42], to five loops in the RI' scheme for the linear covariant gauge for  $13 \leq N_f \leq 16$ .

| Linear Covariant Gauge and mMOM Scheme |      |                |                 |            |                 |
|----------------------------------------|------|----------------|-----------------|------------|-----------------|
|                                        |      | $\bar{\alpha}$ |                 | [42]       |                 |
| $N_f$                                  | Loop | $a_\infty$     | $\alpha_\infty$ | $a_\infty$ | $\alpha_\infty$ |
| 8                                      | 2    | 0.049337       | -3.863406       | 0.052219   | -3.795565       |
|                                        | 4    | 0.064323       | -3.359243       | 0.060959   | -3.485534       |
|                                        | 4    | 0.112763       | 0.695049        | 0.363423   | 0.712602        |
|                                        | 5    | 0.046971       | -2.951933       | 0.047937   | -3.192836       |
|                                        | 5    | 0.074205       | 1.170668        | 0.178070   | 1.377827        |
| 9                                      | 2    | 0.046323       | -3.764323       | 0.048504   | -3.705259       |
|                                        | 4    | 0.056983       | -2.993633       | 0.055612   | -3.212828       |
|                                        | 4    | 0.098875       | 0.938167        | 0.164446   | 0.956855        |
|                                        | 5    | 0.042375       | -2.887326       | 0.043123   | -3.003521       |
|                                        | 5    | 0.070268       | 1.213297        | 0.116454   | 1.315030        |
| 10                                     | 2    | 0.042400       | -3.657192       | 0.043898   | -3.608171       |
|                                        | 4    | 0.046825       | -3.006516       | 0.046629   | -3.124397       |
|                                        | 4    | 0.091174       | 1.051338        | 0.132289   | 1.038384        |
|                                        | 5    | 0.038413       | -2.930885       | 0.039060   | -2.975110       |
|                                        | 5    | 0.069282       | 1.186302        | 0.103319   | 1.204261        |
| 11                                     | 2    | 0.037453       | -3.543073       | 0.038351   | -3.505155       |
|                                        | 3    | 0.043328       | -3.551534       | 0.042908   | -3.513882       |
|                                        | 3    | 0.073405       | -3.844154       | 0.093269   | -3.787885       |
|                                        | 3    | 0.313733       | -3.526301       | 0.481048   | -3.475076       |
|                                        | 3    | 0.568583       | 1.968484        | 0.147705   | 1.893386        |
|                                        | 4    | 0.038483       | -3.055520       | 0.038443   | -3.114044       |
|                                        | 4    | 0.086678       | 1.100345        | 0.118918   | 1.056106        |
|                                        | 5    | 0.034366       | -3.013171       | 0.034890   | -3.025124       |
|                                        | 5    | 0.070636       | 1.092494        | 0.096774   | 1.021248        |

Table SM.7: Fixed points solutions for  $a_\infty$  and  $\alpha_\infty$  to the curve  $\gamma_a(a, \bar{\alpha}) = -\gamma_\alpha(a, \bar{\alpha})$ , in the columns headed with  $\bar{\alpha}$  and the corresponding solutions for the fixed points in the  $(a, \alpha)$ -plane given in [42], to five loops in the mMOM scheme for the linear covariant gauge for  $8 \leq N_f \leq 11$ .

| Linear Covariant Gauge and mMOM Scheme |      |                |                 |            |                 |
|----------------------------------------|------|----------------|-----------------|------------|-----------------|
| $N_f$                                  | Loop | $\bar{\alpha}$ |                 | [42]       |                 |
|                                        |      | $a_\infty$     | $\alpha_\infty$ | $a_\infty$ | $\alpha_\infty$ |
| 12                                     | 2    | 0.031475       | -3.424915       | 0.031919   | -3.398484       |
|                                        | 3    | 0.031275       | -3.329545       | 0.031269   | -3.323533       |
|                                        | 3    | 0.310995       | 1.964759        | 0.138858   | 1.925597        |
|                                        | 4    | 0.030877       | -3.101381       | 0.030859   | -3.126726       |
|                                        | 4    | 0.084245       | 1.107651        | 0.112300   | 1.032029        |
|                                        | 5    | 0.029525       | -3.092376       | 0.029873   | -3.093637       |
|                                        | 5    | 0.075199       | 0.899684        | 0.092477   | 0.737912        |
| 13                                     | 2    | 0.024644       | -3.308050       | 0.024812   | -3.292241       |
|                                        | 3    | 0.023188       | -3.213527       | 0.023188   | -3.213214       |
|                                        | 3    | 0.235956       | 1.953417        | 0.133279   | 1.940673        |
|                                        | 4    | 0.023552       | -3.122593       | 0.023543   | -3.131342       |
|                                        | 4    | 0.083423       | 1.081253        | 0.109339   | 0.972815        |
|                                        | 5    | 0.023430       | -3.131575       | 0.023575   | -3.130751       |
|                                        | 5    | 0.089740       | 0.392486        | 0.088935   | 0.273310        |
|                                        | 5    | 0.271334       | -2.184684       | -          | -               |
|                                        | 5    | 0.273565       | -3.447663       | -          | -               |
| 14                                     | 2    | 0.017346       | -3.199477       | 0.017389   | -3.191979       |
|                                        | 3    | 0.016146       | -3.138109       | 0.016146   | -3.138534       |
|                                        | 3    | 0.198961       | 1.935636        | 0.129903   | 1.941314        |
|                                        | 4    | 0.016447       | -3.112174       | 0.016445   | -3.114255       |
|                                        | 4    | 0.084148       | 1.021376        | 0.109027   | 0.877422        |
|                                        | 5    | 0.016525       | -3.119407       | 0.016555   | -3.118834       |
|                                        | 5    | 0.077663       | -3.397949       | 0.083341   | -0.745879       |
| 15                                     | 2    | 0.010064       | -3.105672       | 0.010070   | -3.103310       |
|                                        | 3    | 0.009537       | -3.080460       | 0.009537   | -3.080626       |
|                                        | 3    | 0.176880       | 1.911746        | 0.128198   | 1.929163        |
|                                        | 4    | 0.009636       | -3.076696       | 0.009636   | -3.076936       |
|                                        | 4    | 0.086740       | 0.920434        | 0.111199   | 0.736988        |
|                                        | 5    | 0.009658       | -3.078272       | 0.009660   | -3.078166       |
|                                        | 5    | 0.056517       | -3.737608       | 0.057124   | -3.612651       |
| 16                                     | 2    | 0.003200       | -3.030401       | 0.003200   | -3.030182       |
|                                        | 3    | 0.003138       | -3.027413       | 0.003138   | -3.027421       |
|                                        | 3    | 0.162414       | 1.881766        | 0.127908   | 1.905111        |
|                                        | 4    | 0.003143       | -3.027352       | 0.003143   | -3.027354       |
|                                        | 4    | 0.092274       | 0.755417        | 0.116265   | 0.528607        |
|                                        | 5    | 0.003143       | -3.027378       | 0.003143   | -3.027377       |
|                                        | 5    | 0.049870       | -3.954695       | 0.050584   | -3.866561       |

Table SM.8: Fixed points solutions for  $a_\infty$  and  $\alpha_\infty$  to the curve  $\gamma_a(a, \bar{\alpha}) = -\gamma_\alpha(a, \bar{\alpha})$ , in the columns headed with  $\bar{\alpha}$  and the corresponding solutions for the fixed points in the  $(a, \alpha)$ -plane given in [42], to five loops in the mMOM scheme for the linear covariant gauge for  $12 \leq N_f \leq 16$ .



| Linear Covariant Gauge and MOMg |      |                |                 |            |                 |
|---------------------------------|------|----------------|-----------------|------------|-----------------|
| $N_f$                           | Loop | $\bar{\alpha}$ |                 | [42]       |                 |
|                                 |      | $a_\infty$     | $\alpha_\infty$ | $a_\infty$ | $\alpha_\infty$ |
| 13                              | 3    | 0.025105       | -3.379348       | 0.024398   | -3.342847       |
|                                 | 3    | 0.196880       | 2.321675        | -          | -               |
|                                 | 3    | 0.267479       | 8.862691        | -          | -               |
| 14                              | 3    | 0.014532       | -3.118112       | 0.014243   | -3.058910       |
|                                 | 3    | 0.121576       | 2.347228        | -          | -               |
|                                 | 3    | 0.172941       | 8.930624        | -          | -               |
| 15                              | 2    | 0.016411       | -3.183539       | -          | -               |
|                                 | 2    | 0.061351       | -3.686159       | -          | -               |
|                                 | 3    | 0.008484       | -3.064491       | 0.008466   | -3.056382       |
|                                 | 3    | 0.126552       | 2.347374        | -          | -               |
|                                 | 3    | 0.182164       | 8.975111        | -          | -               |
| 16                              | 2    | 0.003551       | -3.032726       | 0.003551   | -3.032914       |
|                                 | 2    | 0.117979       | -4.087258       | 0.026797   | -4.022330       |
|                                 | 3    | 0.002939       | -3.026351       | 0.002939   | -3.025985       |
|                                 | 3    | 0.309787       | 2.302676        | -          | -               |
|                                 | 3    | 0.433694       | 8.991508        | -          | -               |

Table SM.9: Fixed points solutions for  $a_\infty$  and  $\alpha_\infty$  to the curve  $\gamma_a(a, \bar{\alpha}) = -\gamma_\alpha(a, \bar{\alpha})$ , in the columns headed with  $\bar{\alpha}$  and the corresponding solutions for the fixed points in the  $(a, \alpha)$ -plane given in [42], to three loops in the MOMg scheme for the linear covariant gauge for  $13 \leq N_f \leq 16$ . There were no solutions for  $N_f \leq 12$ .

| Curci-Ferrari Gauge and MOMg Scheme |      |                |                 |            |                 |
|-------------------------------------|------|----------------|-----------------|------------|-----------------|
| $N_f$                               | Loop | $\bar{\alpha}$ |                 | [42]       |                 |
|                                     |      | $a_\infty$     | $\alpha_\infty$ | $a_\infty$ | $\alpha_\infty$ |
| 16                                  | 2    | 0.009173       | -6.053827       | -          | -               |
|                                     | 2    | 0.035777       | -6.209934       | -          | -               |
|                                     | 3    | 0.003378       | -5.945622       | 0.003108   | -5.886007       |
|                                     | 3    | 0.036989       | 2.678712        | -          | -               |
|                                     | 3    | 0.048060       | 8.736020        | 0.004759   | 10.293237       |

Table SM.10: Fixed points solutions for  $a_\infty$  and  $\alpha_\infty$  to the curve  $\gamma_a(a, \bar{\alpha}) = -\gamma_\alpha(a, \bar{\alpha})$ , in the columns headed with  $\bar{\alpha}$  and the corresponding solutions for the fixed points in the  $(a, \alpha)$ -plane given in [42], to three loops in the MOMg scheme for the Curci-Ferrari gauge for  $N_f = 16$ . There were no solutions for  $N_f \leq 15$ .

| MAG and MOMg Scheme |      |                |                 |            |                 |
|---------------------|------|----------------|-----------------|------------|-----------------|
|                     |      | $\bar{\alpha}$ |                 | [42]       |                 |
| $N_f$               | Loop | $a_\infty$     | $\alpha_\infty$ | $a_\infty$ | $\alpha_\infty$ |
| 8                   | 2    | 0.213988       | -5.661265       | -          | -               |
|                     | 2    | 0.141770       | -5.630143       | -          | -               |
| 10                  | 2    | 0.097441       | -5.611039       | 0.081771   | -4.742280       |
| 11                  | 2    | 0.068040       | -5.598369       | 0.060657   | -4.773577       |
|                     | 3    | 0.118059       | -5.407101       | 0.026190   | -4.789249       |
|                     | 3    | 0.706631       | 1.750852        | -          | -               |
| 12                  | 2    | 0.047296       | -5.589429       | 0.043307   | -4.932430       |
|                     | 3    | 0.039394       | -5.289562       | 0.021171   | -4.968311       |
|                     | 3    | 0.196905       | 1.752856        | -          | -               |
| 13                  | 2    | 0.031943       | -5.582813       | 0.029800   | -5.120744       |
|                     | 3    | 0.026488       | -5.339342       | 0.016638   | -5.169138       |
|                     | 3    | 0.146748       | 1.768290        | -          | -               |
| 14                  | 2    | 0.020151       | -5.577730       | 0.019126   | -5.302003       |
|                     | 3    | 0.017437       | -5.432707       | 0.012327   | -5.355909       |
|                     | 3    | 0.125103       | 1.781890        | -          | -               |
| 15                  | 2    | 0.010821       | -5.573710       | 0.010462   | -5.453155       |
|                     | 3    | 0.009871       | -5.516841       | 0.007915   | -5.497120       |
|                     | 3    | 0.113047       | 1.787407        | -          | -               |
| 16                  | 2    | 0.003264       | -5.570453       | 0.003223   | -5.550742       |
|                     | 3    | 0.003158       | -5.563799       | 0.002925   | -5.562587       |
|                     | 3    | 0.105646       | 1.781036        | -          | -               |

Table SM.11: Fixed points solutions for  $a_\infty$  and  $\alpha_\infty$  to the curve  $\alpha\gamma_a(a, \bar{\alpha}) = -\alpha\gamma_\alpha(a, \bar{\alpha})$ , in the columns headed with  $\bar{\alpha}$  and the corresponding solutions for the fixed points in the  $(a, \alpha)$ -plane given in [42], to three loops in the MOMg scheme for the MAG for various values of  $N_f \leq 16$ .

| Linear Covariant Gauge and MOMc Scheme |      |                |                 |            |                 |
|----------------------------------------|------|----------------|-----------------|------------|-----------------|
|                                        |      | $\bar{\alpha}$ |                 | [42]       |                 |
| $N_f$                                  | Loop | $a_\infty$     | $\alpha_\infty$ | $a_\infty$ | $\alpha_\infty$ |
| 8                                      | 2    | 0.048612       | -5.154921       | 0.028350   | -5.979315       |
|                                        | 3    | 0.048609       | -5.707495       | 0.105376   | -3.505933       |
| 9                                      | 2    | 0.048163       | -4.934829       | 0.030157   | -5.662741       |
|                                        | 3    | 0.053677       | -5.315762       | 0.069807   | -3.572069       |
| 10                                     | 2    | 0.046691       | -4.681645       | 0.031863   | -5.305495       |
|                                        | 3    | 0.050995       | -4.558892       | 0.051534   | -3.505080       |
|                                        | 3    | 0.190699       | -5.984101       | 0.144252   | 1.712801        |
|                                        | 3    | 0.269098       | -4.957579       | -          | -               |
|                                        | 3    | 0.439956       | 1.828283        | -          | -               |
| 11                                     | 2    | 0.043580       | -4.388445       | 0.033011   | -4.893063       |
|                                        | 3    | 0.039759       | -3.867571       | 0.039651   | -3.389029       |
|                                        | 3    | 0.215208       | 1.838060        | 0.127850   | 1.773389        |
| 12                                     | 2    | 0.038072       | -4.054732       | 0.032458   | -4.413214       |
|                                        | 3    | 0.030626       | -3.490380       | 0.030606   | -3.279886       |
|                                        | 3    | 0.154609       | 1.842387        | 0.117718   | 1.815119        |
| 13                                     | 2    | 0.029879       | -3.703578       | 0.028198   | -3.894191       |
|                                        | 3    | 0.022968       | -3.279928       | 0.022969   | -3.195200       |
|                                        | 3    | 0.125615       | 1.846215        | 0.111195   | 1.840240        |
| 14                                     | 2    | 0.020190       | -3.391508       | 0.019968   | -3.455109       |
|                                        | 3    | 0.016056       | -3.158994       | 0.016059   | -3.131502       |
|                                        | 3    | 0.108470       | 1.849745        | 0.107062   | 1.849988        |
| 15                                     | 2    | 0.010998       | -3.167542       | 0.010986   | -3.179697       |
|                                        | 3    | 0.009509       | -3.084201       | 0.009509   | -3.078808       |
|                                        | 3    | 0.097150       | 1.852029        | 0.104715   | 1.844808        |
| 16                                     | 2    | 0.003287       | -3.036419       | 0.003287   | -3.037061       |
|                                        | 3    | 0.003136       | -3.027518       | 0.003136   | -3.027336       |
|                                        | 3    | 0.089172       | 1.851880        | 0.103864   | 1.824430        |

Table SM.12: Fixed points solutions for  $a_\infty$  and  $\alpha_\infty$  to the curve  $\gamma_a(a, \bar{\alpha}) = -\gamma_\alpha(a, \bar{\alpha})$ , in the columns headed with  $\bar{\alpha}$  and the corresponding solutions for the fixed points in the  $(a, \alpha)$ -plane given in [42], to three loops in the MOMc scheme for the linear covariant gauge for  $8 \leq N_f \leq 16$ .

| Curci-Ferrari Gauge and MOMc Scheme |      |                |                 |            |                 |
|-------------------------------------|------|----------------|-----------------|------------|-----------------|
|                                     |      | $\bar{\alpha}$ |                 | [42]       |                 |
| $N_f$                               | Loop | $a_\infty$     | $\alpha_\infty$ | $a_\infty$ | $\alpha_\infty$ |
| 8                                   | 2    | 0.018749       | -6.443161       | 0.020025   | -6.305377       |
| 9                                   | 2    | 0.019132       | -6.287599       | 0.020001   | -6.195104       |
| 10                                  | 2    | 0.019333       | -6.124274       | 0.019717   | -6.083107       |
|                                     | 3    | 0.047556       | -1.217320       | 0.060714   | -3.328911       |
|                                     | 3    | 0.057629       | 1.101744        | 0.077080   | 1.908693        |
| 11                                  | 2    | 0.019164       | -5.958296       | 0.019038   | -5.972364       |
|                                     | 2    | 3.888091       | 2.460962        | 0.251163   | 2.007962        |
|                                     | 3    | 0.041375       | -2.702045       | 0.051508   | -3.611843       |
|                                     | 3    | 0.064300       | 1.887687        | 0.072290   | 2.050258        |
| 12                                  | 2    | 0.018317       | -5.802534       | 0.017776   | -5.868665       |
|                                     | 2    | 0.786507       | 2.478912        | 0.181025   | 2.138558        |
|                                     | 3    | 0.037520       | -3.510581       | 0.043848   | -3.909767       |
|                                     | 3    | 0.070687       | 2.162088        | 0.069815   | 2.152213        |
| 13                                  | 2    | 0.016389       | -5.682308       | 0.015704   | -5.782642       |
|                                     | 2    | 0.439549       | 2.520580        | 0.141722   | 2.275676        |
|                                     | 3    | 0.033847       | -4.116816       | 0.036699   | -4.244411       |
|                                     | 3    | 0.079317       | 2.276119        | 0.069084   | 2.217748        |
| 14                                  | 2    | 0.013097       | -5.633415       | 0.012603   | -5.732572       |
|                                     | 2    | 0.306418       | 2.576379        | 0.116851   | 2.413714        |
|                                     | 3    | 0.028567       | -4.674655       | 0.028567   | -4.674679       |
|                                     | 3    | 0.093797       | 2.293968        | 0.069941   | 2.248236        |
| 15                                  | 2    | 0.008532       | -5.687768       | 0.008357   | -5.747686       |
|                                     | 2    | 0.236119       | 2.640432        | 0.099800   | 2.549312        |
|                                     | 3    | 0.014106       | -5.443902       | 0.014116   | -5.411305       |
|                                     | 3    | 0.130792       | 2.217082        | 0.072570   | 2.242597        |
| 16                                  | 2    | 0.003028       | -5.863149       | 0.003018   | -5.873459       |
|                                     | 2    | 0.192689       | 2.709119        | 0.087420   | 2.680663        |
|                                     | 3    | 0.003389       | -5.849803       | 0.003391   | -5.848457       |
|                                     | 3    | 0.125579       | -4.426388       | 0.077644   | 2.196108        |

Table SM.13: Fixed points solutions for  $a_\infty$  and  $\alpha_\infty$  to the curve  $\gamma_a(a, \bar{\alpha}) = -\gamma_\alpha(a, \bar{\alpha})$ , in the columns headed with  $\bar{\alpha}$  and the corresponding solutions for the fixed points in the  $(a, \alpha)$ -plane given in [42], to three loops in the MOMc scheme for the Curci-Ferrari gauge for  $8 \leq N_f \leq 16$ .

| MAG and MOMc Scheme |      |                |                 |            |                 |
|---------------------|------|----------------|-----------------|------------|-----------------|
|                     |      | $\bar{\alpha}$ |                 | [42]       |                 |
| $N_f$               | Loop | $a_\infty$     | $\alpha_\infty$ | $a_\infty$ | $\alpha_\infty$ |
| 8                   | 2    | 0.113864       | -5.618117       | 0.033217   | -8.455727       |
|                     | 2    | 16.697744      | -12.764998      | -          | -               |
|                     | 3    | 0.061924       | -1.799962       | 0.077117   | -1.000791       |
|                     | 3    | 0.108430       | 6.022244        | -          | -               |
| 9                   | 2    | 0.088606       | -5.607232       | 0.033833   | -8.143603       |
|                     | 2    | 17.430739      | -13.080884      | -          | -               |
|                     | 3    | 0.045222       | -3.276219       | -          | -               |
|                     | 3    | 0.103007       | 6.383916        | -          | -               |
| 10                  | 2    | 0.068649       | -5.598631       | 0.034117   | -7.784169       |
|                     | 2    | 18.158166      | -13.394371      | -          | -               |
|                     | 3    | 0.034099       | -4.137704       | -          | -               |
|                     | 3    | 0.099417       | 6.680198        | 0.525666   | -5.116521       |
| 11                  | 2    | 0.052501       | -5.591672       | 0.033655   | -7.364723       |
|                     | 2    | 18.882614      | -13.706575      | 5.519238   | 1.674527        |
|                     | 3    | 0.026572       | -4.674900       | -          | -               |
|                     | 3    | 0.098867       | 6.925672        | -          | -               |
| 12                  | 2    | 0.039178       | -5.585930       | 0.031606   | -6.879356       |
|                     | 2    | 19.606190      | -14.018403      | 1.476988   | 1.916484        |
|                     | 3    | 0.020946       | -5.050909       | -          | -               |
|                     | 3    | 0.102968       | 7.125603        | 0.203684   | -5.644839       |
| 13                  | 2    | 0.028004       | -5.581115       | 0.026761   | -6.364145       |
|                     | 2    | 20.330631      | -14.330603      | 0.806259   | 2.117233        |
|                     | 3    | 0.016309       | -5.322269       | -          | -               |
|                     | 3    | 0.116255       | 7.277971        | 0.152357   | -5.896500       |
| 14                  | 2    | 0.018503       | -5.577020       | 0.019089   | -5.932927       |
|                     | 2    | 21.057391      | -14.643802      | 0.546940   | 2.294665        |
|                     | 3    | 0.012098       | -5.501851       | 0.018678   | -5.773235       |
|                     | 3    | 0.162130       | 7.365506        | 0.118778   | -6.152061       |
| 15                  | 2    | 0.010326       | -5.573497       | 0.010713   | -5.675674       |
|                     | 2    | 21.787699      | -14.958531      | 0.412326   | 2.456372        |
|                     | 3    | 0.007830       | -5.586104       | 0.009926   | -5.607244       |
| 16                  | 2    | 0.003217       | -5.570433       | 0.003263   | -5.575657       |
|                     | 2    | 22.522604      | -15.275241      | 0.330726   | 2.606374        |
|                     | 3    | 0.002920       | -5.580922       | 0.003158   | -5.568650       |

Table SM.14: Fixed points solutions for  $a_\infty$  and  $\alpha_\infty$  to the curve  $\alpha\gamma_a(a, \bar{\alpha}) = -\alpha\gamma_\alpha(a, \bar{\alpha})$ , in the columns headed with  $\bar{\alpha}$  and the corresponding solutions for the fixed points in the  $(a, \alpha)$ -plane given in [42], to three loops in the MOMc scheme for the MAG for  $8 \leq N_f \leq 16$ .

| Linear Covariant Gauge and MOMq Scheme |      |                |                 |            |                 |
|----------------------------------------|------|----------------|-----------------|------------|-----------------|
|                                        |      | $\bar{\alpha}$ |                 | [42]       |                 |
| $N_f$                                  | Loop | $a_\infty$     | $\alpha_\infty$ | $a_\infty$ | $\alpha_\infty$ |
| 8                                      | 3    | 0.115880       | -11.717492      | 0.063541   | -1.624601       |
|                                        | 3    | 0.233342       | -24.505585      | -          | -               |
| 9                                      | 3    | 0.317699       | -5.188818       | 0.053412   | -1.989647       |
| 10                                     | 3    | 0.056493       | -4.389949       | 0.045054   | -2.279576       |
| 11                                     | 2    | 0.062014       | -5.545270       | -          | -               |
|                                        | 2    | 0.102689       | -7.214720       | -          | -               |
|                                        | 3    | 0.039963       | -3.672932       | 0.037600   | -2.524956       |
| 12                                     | 2    | 0.042552       | -4.498563       | -          | -               |
|                                        | 2    | 0.146842       | -8.171376       | -          | -               |
|                                        | 3    | 0.031102       | -3.341953       | 0.030567   | -2.734762       |
| 13                                     | 2    | 0.029969       | -3.880831       | -          | -               |
|                                        | 2    | 0.195865       | -8.756721       | -          | -               |
|                                        | 3    | 0.023725       | -3.183093       | 0.023664   | -2.903611       |
| 14                                     | 2    | 0.019562       | -3.460982       | 0.019199   | -3.718938       |
|                                        | 2    | 0.263978       | -9.220684       | 0.019368   | -6.388108       |
|                                        | 3    | 0.016742       | -3.111460       | 0.016759   | -3.014525       |
| 15                                     | 2    | 0.010716       | -3.190089       | 0.010692   | -3.221650       |
|                                        | 2    | 0.373168       | -9.619659       | 0.015028   | -8.083894       |
|                                        | 3    | 0.009874       | -3.071048       | 0.009880   | -3.052463       |
| 16                                     | 2    | 0.003259       | -3.038829       | 0.003259   | -3.040137       |
|                                        | 2    | 0.585712       | -9.977608       | 0.012174   | -9.486233       |
|                                        | 3    | 0.003189       | -3.026934       | 0.003189   | -3.026384       |

Table SM.15: Fixed points solutions for  $a_\infty$  and  $\alpha_\infty$  to the curve  $\gamma_a(a, \bar{\alpha}) = -\gamma_\alpha(a, \bar{\alpha})$ , in the columns headed with  $\bar{\alpha}$  and the corresponding solutions for the fixed points in the  $(a, \alpha)$ -plane given in [42], to three loops in the MOMq scheme for the linear covariant gauge for  $8 \leq N_f \leq 16$ .

| Curci-Ferrari Gauge and MOMq Scheme |      |                |                 |            |                 |
|-------------------------------------|------|----------------|-----------------|------------|-----------------|
|                                     |      | $\bar{\alpha}$ |                 | [42]       |                 |
| $N_f$                               | Loop | $a_\infty$     | $\alpha_\infty$ | $a_\infty$ | $\alpha_\infty$ |
| 8                                   | 3    | 0.020141       | -16.249293      | 0.054194   | -7.544746       |
|                                     | 3    | 0.037643       | -34.082576      | -          | -               |
| 9                                   | 3    | 0.021760       | -14.654300      | -          | -               |
|                                     | 3    | 0.045826       | -34.124277      | 0.047413   | -7.526249       |
| 10                                  | 3    | 0.023837       | -12.903447      | 0.027602   | 3.319638        |
|                                     | 3    | 0.059737       | -34.166447      | 0.045671   | -3.502277       |
| 11                                  | 3    | 0.026436       | -10.849035      | 0.034823   | -7.634193       |
|                                     | 3    | 0.092892       | -34.292674      | 0.014604   | 5.033905        |
| 12                                  | 3    | 0.028070       | -8.257204       | 0.028725   | -7.821260       |
| 13                                  | 3    | 0.023672       | -6.114185       | 0.024050   | -4.783367       |
| 14                                  | 2    | 0.021557       | -6.743102       | -          | -               |
|                                     | 2    | 0.134778       | -10.646033      | -          | -               |
|                                     | 3    | 0.016978       | -5.454850       | 0.017042   | -5.188757       |
| 15                                  | 2    | 0.011080       | -6.009784       | 0.011080   | -6.011974       |
|                                     | 2    | 6.333439       | -11.592647      | -          | -               |
|                                     | 3    | 0.010027       | -5.555625       | 0.010029   | -5.545351       |
| 16                                  | 2    | 0.003291       | -5.892358       | 0.003291   | -5.890246       |
|                                     | 3    | 0.003212       | -5.849248       | 0.003212   | -5.850425       |

Table SM.16: Fixed points solutions for  $a_\infty$  and  $\alpha_\infty$  to the curve  $\gamma_a(a, \bar{\alpha}) = -\gamma_\alpha(a, \bar{\alpha})$ , in the columns headed with  $\bar{\alpha}$  and the corresponding solutions for the fixed points in the  $(a, \alpha)$ -plane given in [42], to three loops in the MOMc scheme for the Curci-Ferrari gauge for  $8 \leq N_f \leq 16$ .

| MAG and MOMq Scheme |      |                |                 |            |                 |
|---------------------|------|----------------|-----------------|------------|-----------------|
| $N_f$               | Loop | $\bar{\alpha}$ |                 | [42]       |                 |
|                     |      | $a_\infty$     | $\alpha_\infty$ | $a_\infty$ | $\alpha_\infty$ |
| 8                   | 2    | 0.166338       | -5.640731       | -          | -               |
|                     | 2    | 22.822104      | -15.404312      | -          | -               |
|                     | 3    | 0.063492       | 0.125147        | 0.067519   | -0.911374       |
| 9                   | 2    | 0.117616       | -5.619734       | -          | -               |
|                     | 2    | 23.798553      | -15.825116      | -          | -               |
|                     | 3    | 0.055214       | -1.260495       | 0.054006   | -0.667233       |
| 10                  | 2    | 0.084917       | -5.605642       | -          | -               |
|                     | 2    | 24.743471      | -16.232332      | -          | -               |
|                     | 3    | 0.046418       | -2.553095       | 0.049928   | -5.130987       |
| 11                  | 2    | 0.061529       | -5.595563       | -          | -               |
|                     | 2    | 25.663684      | -16.628901      | -          | -               |
|                     | 3    | 0.038600       | -3.525047       | 0.040453   | -5.311340       |
| 12                  | 2    | 0.043999       | -5.588008       | -          | -               |
|                     | 2    | 26.564366      | -17.017053      | -          | -               |
|                     | 3    | 0.031364       | -4.261418       | 0.032062   | -5.449734       |
| 13                  | 2    | 0.030386       | -5.582141       | -          | -               |
|                     | 2    | 27.449548      | -17.398525      | -          | -               |
|                     | 3    | 0.024236       | -4.822255       | 0.024313   | -5.538771       |
| 14                  | 2    | 0.019513       | -5.577456       | 0.018512   | -6.159115       |
|                     | 2    | 28.322438      | -17.774700      | 0.014689   | -12.833072      |
|                     | 3    | 0.017062       | -5.220839       | 0.016971   | -5.576405       |
| 15                  | 2    | 0.010634       | -5.573629       | 0.010513   | -5.718031       |
|                     | 2    | 29.185645      | -18.146702      | 0.011319   | -15.419119      |
|                     | 3    | 0.009967       | -5.460114       | 0.009925   | -5.576887       |
| 16                  | 2    | 0.003246       | -5.570446       | 0.003244   | -5.578975       |
|                     | 2    | 30.041314      | -18.515456      | 0.009224   | -17.653356      |
|                     | 3    | 0.003194       | -5.559774       | 0.003192   | -5.567723       |

Table SM.17: Fixed points solutions for  $a_\infty$  and  $\alpha_\infty$  to the curve  $\alpha\gamma_a(a, \bar{\alpha}) = -\alpha\gamma_\alpha(a, \bar{\alpha})$ , in the columns headed with  $\bar{\alpha}$  and the corresponding solutions for the fixed points in the  $(a, \alpha)$ -plane given in [42], to three loops in the MOMc scheme for the MAG for  $8 \leq N_f \leq 16$ .
